# Supplementary material for: Fast and Memory-Efficient Neural Code Completion
Source: arXiv:2004.13651 source file (2021-03-16)
Supplement: Supplementary file 1 [file appendix.tex]

\section{Implementation Concerns}
During training, we want to compute representations of the candidate completion targets
provided by \candidateProvider for each sample in a minibatch and then score these representations
against the output of \contextEncoder for each of the corresponding contexts.
One problem we encounter when using the static analysis-based candidate provider \staticAnalysisProvider
is that the number of candidate targets, \ie $|\candidateProvider(\vect{t}_{\text{cx}})|$,
varies widely for different contexts $\vect{t}_{\text{cx}}$. One option would be to pad up to a
maximum number of suggestions, but given the severe
skew in the distribution of the number of suggestions from \candidateProvider for different completion contexts,
this would lead to wasted computational effort.
We overcome this by flattening the
suggestions along the batch dimension, feeding them into the token encoder together with
a complimentary tensor that encodes the origin index of each suggestion. This
allows us to perform distributed scatter-style operations\footnote{For example
\href{https://www.tensorflow.org/api_docs/python/tf/math/unsorted_segment_sum}{\code{unsorted\_segment\_sum}} in TensorFlow,
and \href{https://pytorch.org/docs/master/tensors.html\#torch.Tensor.scatter\_add\_}{\code{scatter\_add\_}} in PyTorch.}
and efficiently compute \autoref{eqn:prob} across the examples in the
training minibatch without padding. At test time, this problem vanishes since
no batching is required.
